# Supplementary material for: Sign-Agnostic Implicit Learning of Surface Self-Similarities for Shape Modeling and Reconstruction from Raw Point Clouds
Source: arXiv:2012.07498 source file (2021-06-08)
Supplement: Supplementary file 8 [file supp.tex]

\clearpage

%%%%%%%%%%%%%%%%%%%%%%%%%%%%%%%%%%%%%%%%%%%%%%%%%%%%%%%%%%%%
%%%%%%%%%%%%%%%%%%%%%%% Sphere fitting %%%%%%%%%%%%%%%%%%%%%
%%%%%%%%%%%%%%%%%%%%%%%%%%%%%%%%%%%%%%%%%%%%%%%%%%%%%%%%%%%%

\section{Least Squares Method for Sphere}
In this section, we will introduce how to estimate the center $\bar{\bm{t}}$ and the radius $\bar{\bm{r}}$ given the observed points $\{{\bm{p}}\}$ with least squares method.
We are actually going to solve the problem of equations as follows,
\begin{equation}\label{EqnLeastSquareFitting}
    \begin{split}
        & \qquad\qquad\qquad (\bar{r}, \bar{\bm{t}}) = \arg\min_{\bar{r}', \bar{\bm{t}}'} \|Ab-Y\|, \\
        &Y=\left[
    \begin{matrix}
        ({\bm{p}_1^{1}})^2 & ({\bm{p}_1^{1}})^2 & ({\bm{p}_1^{1}})^2 \\
        \vdots & \vdots & \vdots \\
        ({\bm{p}_1^{n}})^2 & ({\bm{p}_1^{n}})^2 & ({\bm{p}_1^{n}})^2
     \end{matrix}
     \right],
    b=\left[
    \begin{matrix}
        \bar{\bm{t}}_1'\\
        \bar{\bm{t}}_2'\\
        \bar{\bm{t}}_3'\\
        \|\bar{\bm{t}}\|_2^2+\bar{r}'^2
    \end{matrix}
     \right],\\
    &A=\left[
        \begin{matrix}
            2\bm{p}_1^{1} & 2\bm{p}_2^{1} & 2\bm{p}_3^{1} & 1 \\
            \vdots & \vdots & \vdots & \vdots \\
            2\bm{p}_1^{n} & 2\bm{p}_2^{n} & 2\bm{p}_3^{n} & 1 \\
         \end{matrix}
         \right],
    \end{split}
\end{equation}

\section{Generation of Minimum Spanning Tree}
In this section, we will introduce how to generate a Minimum Spanning Tree (MST).
Simply put, MST grows a set $\mathcal{V}_{\textrm{MST}}$ as a tree by selecting the vertices from $\mathcal{V}$. Starting from $\mathcal{V}_{\textrm{MST}} = \emptyset$, MST randomly selects a vertex from $\mathcal{V}$, denoted as $v_1$, and assigns $h(v_1) = 1$.
The tree then grows iteratively by selecting from $\mathcal{V} / \mathcal{V}_{\textrm{MST}}$ the vertex that has the lowest edge weight in $\mathcal{W}$ to connect with any vertex in $\mathcal{V}_{\textrm{MST}}$, and ensures not to form a closed loop with those previous selected edges.
In any iteration, denote the selected edge as $e_{i, j}$, $v_j \in \mathcal{V} / \mathcal{V}_{\textrm{MST}}$ is the selected vertex and $v_i$ is the corresponding vertex already in $\mathcal{V}_{\textrm{MST}}$; we set $h(v_j) = h(v_i)$ when $w_{i, j}^1(e_{i,j}) < w_{i, j}^0(e_{i,j})$, and $h(v_j) = - h(v_i)$ otherwise.
The tree is spanned until $|\mathcal{V}_{\textrm{MST}}| = |\mathcal{V}|$, and we have the signs $\{ h(v_i) \}_{i=1}^N$ determined for all the vertices by then.

%%%%%%%%%%%%%%%%%%%%%%%%%%%%%%%%%%%%%%%%%%%%%%%%%%%%%%%%%%%%
%%%%%%%%%%%%%%%%%%%%%%%%%%% Proof %%%%%%%%%%%%%%%%%%%%%%%%%%
%%%%%%%%%%%%%%%%%%%%%%%%%%%%%%%%%%%%%%%%%%%%%%%%%%%%%%%%%%%%

\section{Proof of Corollary \ref{InitCol}}
%\begin{corollary}
%Let $f:\mathbb{R}^{3+d}\to\mathbb{R}$ be a $l$-layer MLP with ReLU activation $\nu$ as the activation functions.
%That is, $f(\bm{p},\bm{z})=\bm{w}^T\nu(\bm{W}^{l}(\cdots\nu(\bm{W}_{\bm{p}}^{1}\bm{p}+\bm{W}_{\bm{z}}^{1}\bm{z}+\bm{b}^{1}))+\bm{b}^{l})+c$, where $\bm{W}_{\bm{p}}^{1}\in\mathbb{R}^{d^{1}_{out}\times 3}$ and $\bm{W}_{\bm{z}}^{1}\in\mathbb{R}^{d^{1}_{out}\times d}$ denote the weight matrix of the first layer, $\bm{b}^{1}\in\mathbb{R}^{d^{1}_{out}}$ denotes the bias of the first layer; $\bm{W}^{l}\in\mathbb{R}^{d^{l}_{out}\times d^{l}_{in}}$ and $\bm{b}^{l}\in\mathbb{R}^{d^{l}_{out}}$ denote and the learnable parameters of the $l^{th}$-layer; $\bm{w}\in\mathbb{R}^{d_{out}}$, $c\in\mathbb{R}$ are the learnable parameters of the last layer; $\bm{p}\in\mathbb{R}^3$ is the input point, and $\bm{z}\in\mathbb{R}^{d}$ is the latent code, which is i.i.d. normal $\mathcal{N}(0,\sigma_{z}^2)$.
%Let $\bm{w}=\frac{\sqrt{2\pi}}{\sigma d_{out}}\bm{1}$, $c=-\bar{r}$, $\bar{r}>0$, let all entries of $\bm{W}^{i}$ ($2\leq i\leq l$) and $\bm{W}_{\bm{p}}^{1}$ are i.i.d. normal $\mathcal{N}(0,\sigma^2)$, and let $b_i=0$ ($2\leq i\leq l$).
%If $\bm{W}_{\bm{z}}^{1}=\bm{W}_{\bm{p}}^{1}[\bm{I}\in\mathbb{R}^{3\times 3}, \bm{0}\in\mathbb{R}^{3\times d}]$ $\bm{b}_1=\bm{W}_{\bm{p}}^{1}\bar{\bm{t}}$, then $\lim_{\sigma\to 0} f(x) = \|\bm{p}-\bar{\bm{t}}\| - \bar{r}$.
%That is, $f$ is approximately the signed distance function to a 3D sphere of radius $\bar{r}$, centered at the $\bar{\bm{t}}$.
%\end{corollary}

\begin{proof}
Note that plugging $\bm{W}_2$, $b$ in $f$ we get $f(\bm{p},\bm{z})=\bm{w}^T\nu(\bm{W}_1(\bm{p}+\bm{z}_{[1:3]}+\bar{\bm{t}}))+c$.
Let $\bm{x}\in\mathbb{R}^3 = \bm{p}+\bm{z}_{[1:3]}+\bar{\bm{t}}$ and further plugging $w$, $c$ in $f$, we get $f(x) = \frac{\sqrt{2}\pi}{\sigma d^{out}}\sum_{i=1}^{d^{out}}\nu(\bm{w}_{1,i}\cdot\bm{x})-r$, where $\bm{w}_{1,i}$ is the $i^{th}$ row of $\bm{W}_1$.
Let $\mu$ denotes the density of multivariate normal distribution $\mathcal{N}(0,\sigma \bm{I}_d)$.
The first term converges to $\|\bm{x}\|$, which is a direct consequence following Theorem $2$ in \cite{Atzmon2020_SAL}.
In other words,  $f(x) \approx \|\bm{p}-\bar{\bm{t}}+\bm{z}_{[1:3]}\| - \bar{r} \approx \|\bm{p}-\bar{\bm{t}}\| - \bar{r}$.
Note that to make the assumption of $\bm{b}$ and $\bm{W}_2$ to be true, the dimension of $d^{out}$ should satisfy $|d^{out}|\geq3$ to solve the system of equations.
\end{proof}


%%%%%%%%%%%%%%%%%%%%%%%%%%%%%%%%%%%%%%%%%%%%%%%%%%%%%%%%%%%%
%%%%%%%%%%%%%%%%%% More Quality Results %%%%%%%%%%%%%%%%%%%%
%%%%%%%%%%%%%%%%%%%%%%%%%%%%%%%%%%%%%%%%%%%%%%%%%%%%%%%%%%%%

\section{More Quality Results} \label{app:quality}
We show more quality results in this section.

\input{figures/fig_comp_supp}




%%%%%%%%%%%%%%%%%%%%%%%%%%%%%%%%%%%%%%%%%%%%%%%%%%%%%%%%%%%%
%%%%%%%%%%%%%%%%%%%%%% Ablation Study %%%%%%%%%%%%%%%%%%%%%%
%%%%%%%%%%%%%%%%%%%%%%%%%%%%%%%%%%%%%%%%%%%%%%%%%%%%%%%%%%%%

\section{Ablation Study}
To show the efficiency of each component in our pipeline, we conduct ablation studies in this section.

\nothing{
\vspace{0.1cm}
\noindent\textbf{Adaptive cells}
This experiment is to validate the performance improvement brought by self-adapting cells presented in Section \ref{sec:cells_adapting}.
We compare our approach with the one without adapting cells' centers ${\{\bm{c}_i\}}_{i=1}^n$ and scales ${\{s_i\}}_{i=1}^n$.
Concretely, we initialize centers ${\{\bm{c}_i\}}_{i=1}^n$ and scales ${\{s_i\}}_{i=1}^n$ to form a regular arrangement of cells and parameters ${\{\bm{c}_i\}}_{i=1}^n$ and ${\{s_i\}}_{i=1}^n$ are fixed during fitting, which is the method described in \cite{}.
}

\vspace{0.1cm}
\noindent\textbf{Initialization for Signed Solutions -- }
To evaluate the advantages of our proposed initialization for signed solution presented in Section \ref{sec:method_sign_agnostic}, we conduct experiments with and without it.
As can be seen in Figure \ref{fig:abla_init}, replacing our geometric initialization with random initialization, the reconstruction results will fall into unsigned solution.
\input{figures/fig_ablation_geo_init}


\vspace{0.1cm}
\noindent\textbf{Local Sign Flipping -- }
To demonstrate the effectiveness of the local sign flipping strategy presented in Section \ref{sec:method_post_opt},
we comparing between with and without using the proposed flipping strategy.
As can be seen in Figure \ref{fig:abla_sign_flip}, without using local sign flipping strategy, square grids would appear after Marching Cubes \cite{lorensen1987marching}, because of the inconsistency of sign between different subfields.

\vspace{0.1cm}
\noindent\textbf{Interpolation of Local Fields --}
The validity of the proposed interpolation of local fields can be checked by substituting interpolation by max pooling or average pooling.
Without interpolating the overlapping cells, the implicit fields are inconsistent near the boundaries, and results in uneven surface as shown in Figure \ref{fig:abla_inter}.

\input{figures/fig_ablation_interp}
